# Supplementary material for: Global phase diagram of a three dimensional dirty topological superconductor
Source: arXiv:1604.01390 ancillary file (2017-06-01)
Supplement: Supplementary file 1 [file TSCDisorder_Supplementary.pdf]

# Supplementary Materials for "*Global Phase Diagram of a Three Dimensional Dirty Topological Superconductor*"

Bitan Roy, Yahya Alavirad, and Jay D. Sau
*Condensed Matter Theory Center, Department of Physics, University of Maryland, College Park, MD 20742, USA*
(Dated: June 1, 2017)

The Supplementary Material contains:

1. Symmetry of a class DIII system and the scaling analysis near BCS-BEC quantum critical point (QCP),
2. Leading order renormalization group (RG) analysis with all possible disorder (including magnetic disorder),
3. RG calculation for mass (both scalar and pseudo-scalar) disorder beyond the leading order,
4. Additional numerical results across topological-trivial superconductors and metal-insulator transitions,
5. Representation of general odd-parity pairing in $Cu_xBi_2Se_3$ in band basis (including nematic superconductor).

## I. SYMMETRY, SCALING AND DISORDER

The reduced BCS Hamiltonian for class DIII is given by $H=\sum_{\mathbf{k}} \Psi^\dagger_{\mathbf{k}} \hat{H}_{\mathbf{k}} \Psi_{\mathbf{k}}$, where the four component spinor is defined as $\Psi^\dagger_{\mathbf{k}} = \left( c^\ast_{\uparrow,\mathbf{k}}, c^\ast_{\downarrow,\mathbf{k}}, c_{\downarrow,-\mathbf{k}}, -c_{\uparrow,-\mathbf{k}} \right)$. The Hamiltonian operator is

$$\hat{H}_{\mathbf{k}} = \left( \frac{\mathbf{k}^2}{2m_\ast} - \mu \right) \gamma_0 + \left( \frac{\Delta_t}{k_F} \right) i\gamma_0 \gamma_j k_j, \tag{1}$$

is invariant under the reversal of time ($\mathcal{T}$), where $\mathcal{T}=\gamma_1\gamma_3 K$ and $K$ is the complex conjugation, and in addition also possesses an emergent parity ($\mathcal{P}$) symmetry, under which $\mathbf{k}\to-\mathbf{k}$ and $\Psi_{\mathbf{k}} \to \gamma_0 \Psi_{-\mathbf{k}}$. The $\gamma$ matrices are defined as $\gamma_0=\tau_3\otimes\sigma_0$, $\gamma_5=\tau_1\otimes\sigma_0$, $\gamma_j=\tau_2\otimes\sigma_j$ for $j=1,2,3$. Two sets of Pauli matrices $\boldsymbol{\tau}$ and $\boldsymbol{\sigma}$ respectively operate on Nambu and spin indices. In addition, at the BCS-BEC QCP system enjoys an emergent continuous symmetry under the global chiral rotation $\Psi \to e^{i\theta\gamma_5}\,\Psi$. We here change the notation $\tilde{\mu}\to\mu$ from the main part of the paper for notational simplicity.

All together one can write down four types of elastic scatterers and their effect can be captured by the Hamiltonian

$$H_D = V_V(\mathbf{x})\gamma_0 + V_R(\mathbf{x})\gamma_5 + V_I(\mathbf{x}) i\gamma_0\gamma_5 + V^j_M(\mathbf{x}) i\gamma_5\gamma_j. \tag{2}$$

Physical meaning of each term has explicitly been demonstrated in the main part of the paper, and their transformation under various symmetry operation in displayed in Table I. To understand the influence of randomness near the BCS-BEC QCP (located at $\mu=0$), next we perform disorder averaging to arrive at the imaginary time replicated action

$$\bar{S} = \int d^D\vec{x}d\tau \; \left( \Psi^\dagger_a \left[ -i\partial_\tau + iv\gamma_j\partial_j - (b\partial^2+\mu) \right] \Psi_a \right)_{(\tau,\vec{x})} - \sum \frac{\Delta_N}{2} \int d^D\vec{x}d\tau d\tau' \left( \Psi^\dagger_a N \Psi_a \right)_{(\vec{x},\tau)} \left( \Psi^\dagger_b N \Psi_b \right)_{(\vec{x},\tau')}, \tag{3}$$

where the summation in the last term runs over all possible disorder couplings, $a,b$ are replica indices, $v=\Delta_t/k_F$ is the effective Fermi velocity of BdG quasiparticles, $b=1/(2m_\ast)$ and $D$ is spatial dimensions. Here, $\Delta_N$ is the disorder coupling constant, obatined after performing the disorder average, see Table I. Due to the $z=1$ structure of the theory near the toplogical phase transition, under rescaling of space-time coordinates $(\mathbf{x},\tau)\to e^l(\mathbf{x},\tau)$, which leaves the quadratic part of the replicated action invariant when accompanied by the rescaling of fermionic field $\Psi\to e^{-dl/2}\Psi$. Therefore, the scaling dimensions of various parameter in Eq. (3) are $[v]=0$, $[b]=-1$, $[\mu]=1$, $[\Delta_N]=2-D=-1$ for $D=3$. Therefore, any sufficiently weak disorder is an *irrelevant* perturbation at the BCS-BEC QCP, while $\mu$, $v$ and $b$ are respectively relevant, marginal and irrelevant parameters at this QCP.

| Bilinear | $\mathcal{T}$ | $\mathcal{P}$ | $\mathcal{C}$ | $U_c$ | Disorder average | Physical meaning fermion bilinear |
|---|---|---|---|---|---|---|
| $\Psi^\dagger \gamma_0 \Psi$ | ✓ | ✓ | ✓ | × | $\langle\langle V_0(\mathbf{x}) V_0(\mathbf{x}')\rangle\rangle = \Delta_V \delta^3(\mathbf{x}-\mathbf{x}')$ | random charge impurity |
| $\Psi^\dagger \gamma_5 \Psi$ | ✓ | × | ✓ | ✓ | $\langle\langle V_R(\mathbf{x}) V_R(\mathbf{x}')\rangle\rangle = \Delta_R \delta^3(\mathbf{x}-\mathbf{x}')$ | random $s$-wave pairing (real component) |
| $\Psi^\dagger i\gamma_0\gamma_5 \Psi$ | × | × | ✓ | × | $\langle\langle V_I(\mathbf{x}) V_I(\mathbf{x}')\rangle\rangle = \Delta_I \delta^3(\mathbf{x}-\mathbf{x}')$ | random $s$-wave pairing (imaginary component) |
| $\Psi^\dagger i\gamma_5\gamma_j \Psi$ | × | ✓ | × | × | $\langle\langle V^j_M(\mathbf{x}) V^k_M(\mathbf{x}')\rangle\rangle = \delta_{jk}\Delta_M \delta^3(\mathbf{x}-\mathbf{x}')$ | random magnetic impurity |

Table I: Transformation of various disorder under discrete ($\mathcal{T}$, $\mathcal{P}$, $\mathcal{C}$) and continuous chiral ($U_c$) symmetries, and distribution of disorder. Double angular bracket represents disorder average with Gaussian white noise distribution. Under charge conjugation ($\mathcal{C}$) operation, $\mathcal{C}\Psi^\dagger M \Psi \mathcal{C} = -\Psi^\dagger \mathcal{C} M^\top \mathcal{C} \Psi$, where $\mathcal{C} = \gamma_2$. The left most column shows the physical origin of various fermion bilinears.

## II. RENORMALIZATION GROUP ANALYSIS

In the main part of the paper we reported the RG flow equations of various parameters schematically. We here take the opportunity to display these flow equations in details

$$
\begin{aligned}
\frac{d\Delta_V}{dl} &= -\Delta_V - 2\Delta_V \left[\frac{\Delta_V - \Delta_R - \Delta_I + 3\Delta_M}{1+(b-\mu)^2}\right], \quad \frac{d\Delta_M}{dl} = -\Delta_M + 2\Delta_M \left[\frac{\Delta_V + 3\Delta_R - \Delta_I - \Delta_M}{3[1+(b-\mu)^2]}\right], \\
\frac{d\Delta_R}{dl} &= -\Delta_R + \frac{2\Delta_R}{1+(b-\mu)^2}\left[-\Delta_V + \Delta_R - \Delta_I - 3\Delta_M + 2\frac{\Delta_M^2}{\Delta_R}\right], \quad \frac{d\Delta_I}{dl} = -\Delta_I + 2\Delta_I \left[\frac{\Delta_V + \Delta_R - \Delta_I + 3\Delta_M}{1+(b-\mu)^2}\right], \\
\frac{db}{dl} &= -b, \quad \frac{dv}{dl} = v\left[z - 1 - (\Delta_V + \Delta_R + \Delta_I + 3\Delta_M)\right], \quad \frac{d\mu}{dl} = \mu + \left[\Delta_V - \Delta_R - \Delta_I + 3\Delta_M\right] b, \qquad (4)
\end{aligned}
$$

written in terms of dimensionless variable, $b\Lambda/v \to b$, $\mu/(v\Lambda) \to \mu$, $\Delta_N \Lambda/(2\pi^2 v^2) \to \Delta_N$, after integrating the fast Fourier modes within the shell $\Lambda e^{-l} < |\mathbf{k}| < \Lambda$. The relevant one-loop diagrams are shown in Fig. 1. The marginality condition for the Fermi velocity is maintained in the presence of randomness at the cost of a scale dependent dynamic scaling exponent

$$
z(l) = 1 + \left[\Delta_V(l) + \Delta_R(l) + \Delta_I(l) + 3\Delta_M(l)\right]. \qquad (5)
$$

Notice that the set of flow equations remians closed with two time-reversal symmetry ($\mathcal{T}$) preserving disorder couplings $\Delta_V$ and $\Delta_R$, which is guaranteed from the fact that $\mathcal{T}$ is a bonafide microscopic symmetry for a class DIII system, which in its minimal description (four component Dirac fermion) accommodates only two $\mathcal{T}$ preserving disorder vertices. However, when we account for $\mathcal{T}$-breaking disorder, such as $\Delta_I$ and $\Delta_M$, through loop correction we generate some spurious disorder vertices, which are identically zero due to exact particle-hole symmetry of the problem. Thus, during the process of coarse graining whenever we generate such non-local four-fermion vertex, we neglect their input into the RG equations.

The flow equations for $\Delta_V$ and $\Delta_R$ remain closed under RG and supports (i) a quantum critical point at $b = \mu = \Delta_V = 0$ and $\Delta_R = \Delta_R^* = 1/2$, where the correlation length exponent $\nu = 1$ and dynamic sclaing exponent $z = 3/2$, and (ii) a line of quantum critical point for $\mu = b = 0$ in the $(\Delta_V, \Delta_R)$-plane, determined by the equation $\Delta_R^* = \Delta_V^* + 1/2$, along which $\nu = 1$, but the dynamic scaling exponent varies contonuously according to $z = 3/2 + 2\Delta_V^*$[1].

In the presence of time-reversal-symmetry breaking disorder besides the above two solutions the set of coupled flow equations also supports (iii) a line of critical points in the $(\Delta_R, \Delta_I)$ and $\mu = b = \Delta_V = \Delta_M = 0$ plane determined by $\Delta_R^* = \Delta_I^* + 1/2$, along which the dynamic scaling exponent varies continuously as $z = 3/2 + 2\Delta_I^*$, but the correlation length exponent remains fixed at $\nu = 1$, and (iv) a quantum critical point at $\mu = b = \Delta_V = \Delta_I = 0$ and $\Delta_R^* = 9/10$, $\Delta_M^* = 6/5$, where $\nu = 1$ and $z = 11/2$. The fact that the correlation length exponent $\nu = 1$ at all quantum critical points as well as along the entire line of quantum critical points is, however, only an artifact of one-loop calculation.

## III. BEYOND LEADING ORDER RG ANALYSIS FOR MASS DISORDER

We now comment on possible (putative) origin of mass disorder (arising from random charge impurities in class DIII) driven instability of Dirac femrion into a metallic phase. For this purpose, we consider the flow equation of

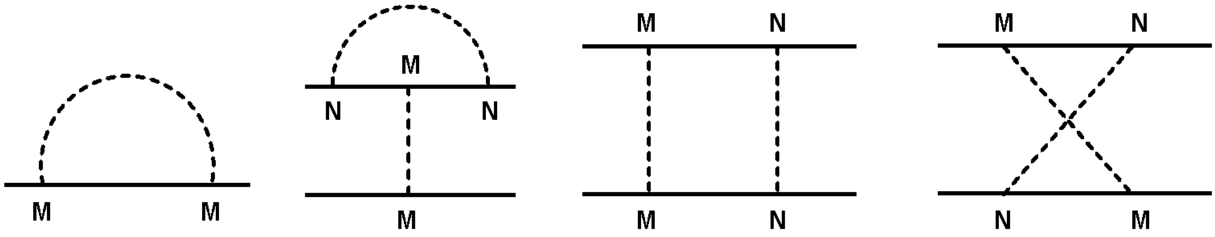


Figure 1: One-loop diagrams leading to the flow equations shown in Eq. (4). Here, M and N are $4 \times 4$ matrices (see Table I).

mass disorder ($\Delta_V$) beyond the leading order, which can be derived from the flow equation of well studied Gross-Neveu model for discrete chiral symmetry breaking mass condensation for massless Dirac fermion in $d$ space-time dimensions[2–5]. The Euclidean (imaginary time) action for such Gross-Neveu model reads as

$$S_{GN} = \int d^d \vec{x} \left[ \bar{\Psi} \left(-i\gamma_\mu \partial_\mu\right) \Psi - g \left(\bar{\Psi}\Psi\right)^2 \right], \tag{6}$$

where $\bar{\Psi} = \Psi^\dagger \gamma_0$ is an independent Grassman variable and $\vec{x}$ corresponds to space-time coordinate. The flow equaition for Gross-Neveu coupling ($g$) is known to three-loop order (we here subscribe to the infra-red flow equation) within the framework of an $\epsilon$-expansion, where $\epsilon = d - 2$, and is given by[2–5]

$$\beta_g = -\epsilon \, g + (n-2) \, g^2 - (n-2) \, g^3 - (n-2)(n-7) \, \frac{g^4}{4}, \tag{7}$$

where $n$ is the number of spinor components. The flow equation of mass disorder, for which the imaginary time replicated action takes the form

$$\bar{S}_D = \int d^D \vec{x} d\tau \, \left( \bar{\Psi}_a \left[-i\partial_\tau \gamma_0 - iv\gamma_j \partial_j\right] \Psi_a \right)_{(x,\tau)} - \frac{\Delta_V}{2} \int d^D \vec{x} d\tau d\tau' \left(\bar{\Psi}_a \Psi_a\right)_{(x,\tau)} \left(\bar{\Psi}_b \Psi_b\right)_{(x,\tau')} \tag{8}$$

where $a$ and $b$ are replica indices and $D$ represents spatial dimensionality of the system, can readily be obtained after setting $n = 0$ (since fermionic bubble does not contribute in the vanishing replica limit[6]) in Eq. (7), leading to

$$\beta_{\Delta_V} = -\epsilon \, \Delta_V - 2 \, \Delta_V^2 + 2 \, \Delta_V^3 - \frac{7}{2} \, \Delta_V^4, \tag{9}$$

where $\epsilon = D - 2$. Such direct mapping between Eqs. (7) and (9) is possible, since the diagramatic contributions from the actions shown in Eqs. (6) and (8) are identical to any order in perturbation theory. Solutions ($\Delta^*_{V,n}$) of the flow equation from Eq. (9) after accounting for perturbative contributions to the $n^{th}$ order ($\propto \Delta_V^{n+1}$) are given by

$$\Delta^*_{V,1} = -\frac{\epsilon}{2} + \mathcal{O}(\epsilon^2), \quad \Delta^*_{V,2} = \frac{1}{2}\left(1 + \sqrt{1+2\epsilon}\right) = 1 + \frac{\epsilon}{2} - \frac{\epsilon^2}{4} + \mathcal{O}(\epsilon^3), \quad \Delta^*_{V,3} = -\frac{\epsilon}{2} + \frac{\epsilon^2}{4} - \frac{\epsilon^3}{32} + \mathcal{O}(\epsilon^4). \tag{10}$$

Although we have expanded $\Delta^*_{V,n}$ in powers of $\epsilon$ for $n = 2$ and 3, such power series expansion is not very well defined, since the radius of convergence of these two series is $\leq 1/2$, as it is evident from $\Delta^*_{V,2}$. However, these three solutions allows us to establish a subtle issue related to mass disorder. Notice that $\Delta^*_{V,1}$ and $\Delta^*_{V,3}$ does not support any critical point since $\Delta^*_{V,1/3} < 0$ for any value of $0 \leq \epsilon \leq 1$. However, two loop RG flow equation supports a quantum critical point at $\Delta_V = \Delta^*_{V,2}$. Therefore, we believe that mass disorder driven instability of massless Dirac femrion into a metallic phase can be addressed appropriately only after accounting for all order perturbation theory. The same sublety arises when one wishes to address possible instability of a Dirac fermion to a metal driven by $\mathcal{P}, \mathcal{T}$-odd mass disorder, which in the BdG Hamiltonian for class DIII system arises from the imaginary component of the $s$-wave pairing.

## IV. ADDITIONAL NUMERICAL RESULTS

We now provide some deatils related to our numerical analysis. The probability that strength of any disorder at a given site is $x\Delta$ follows the standard normal distribution

$$\mathcal{P}(x) = \frac{1}{\sqrt{\pi}} \, \exp\left(-\frac{x^2}{2}\right), \tag{11}$$

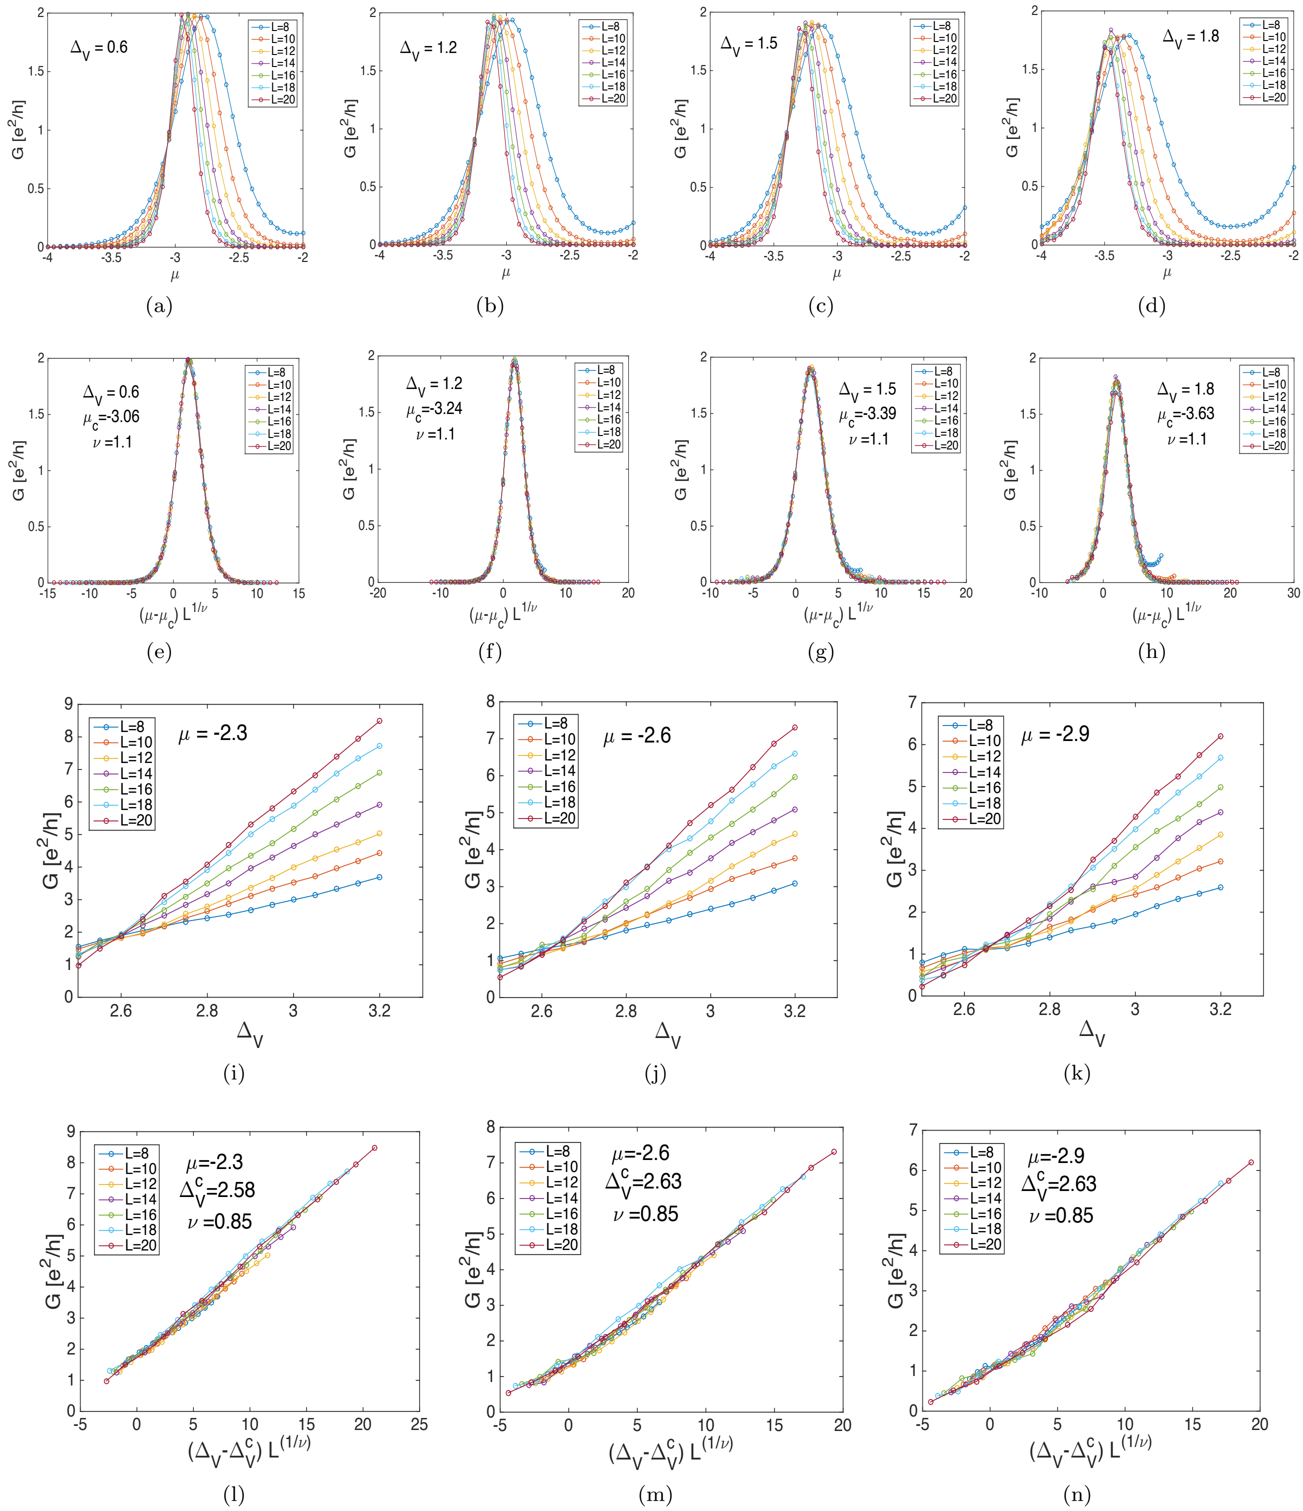


Figure 2: Normalized thermal conductance (NTC) $G$ (in units of $e^2/h$) across thermal insulator-insulator transition (IIT), tuned by random chemical potential (regular Dirac mass disorder) is shown in subfigures (a)-(d). Corresponding data collapses are presented in (e)-(h). NTC across metal-insulator transition (MIT) is shown in subfigures (i)-(k), and associated data collapses across MIT are displayed in (l)-(m). Location of the transition points, best fitting values of $\nu$ across IIT and MIT, system sizes are quoted inside the figures.

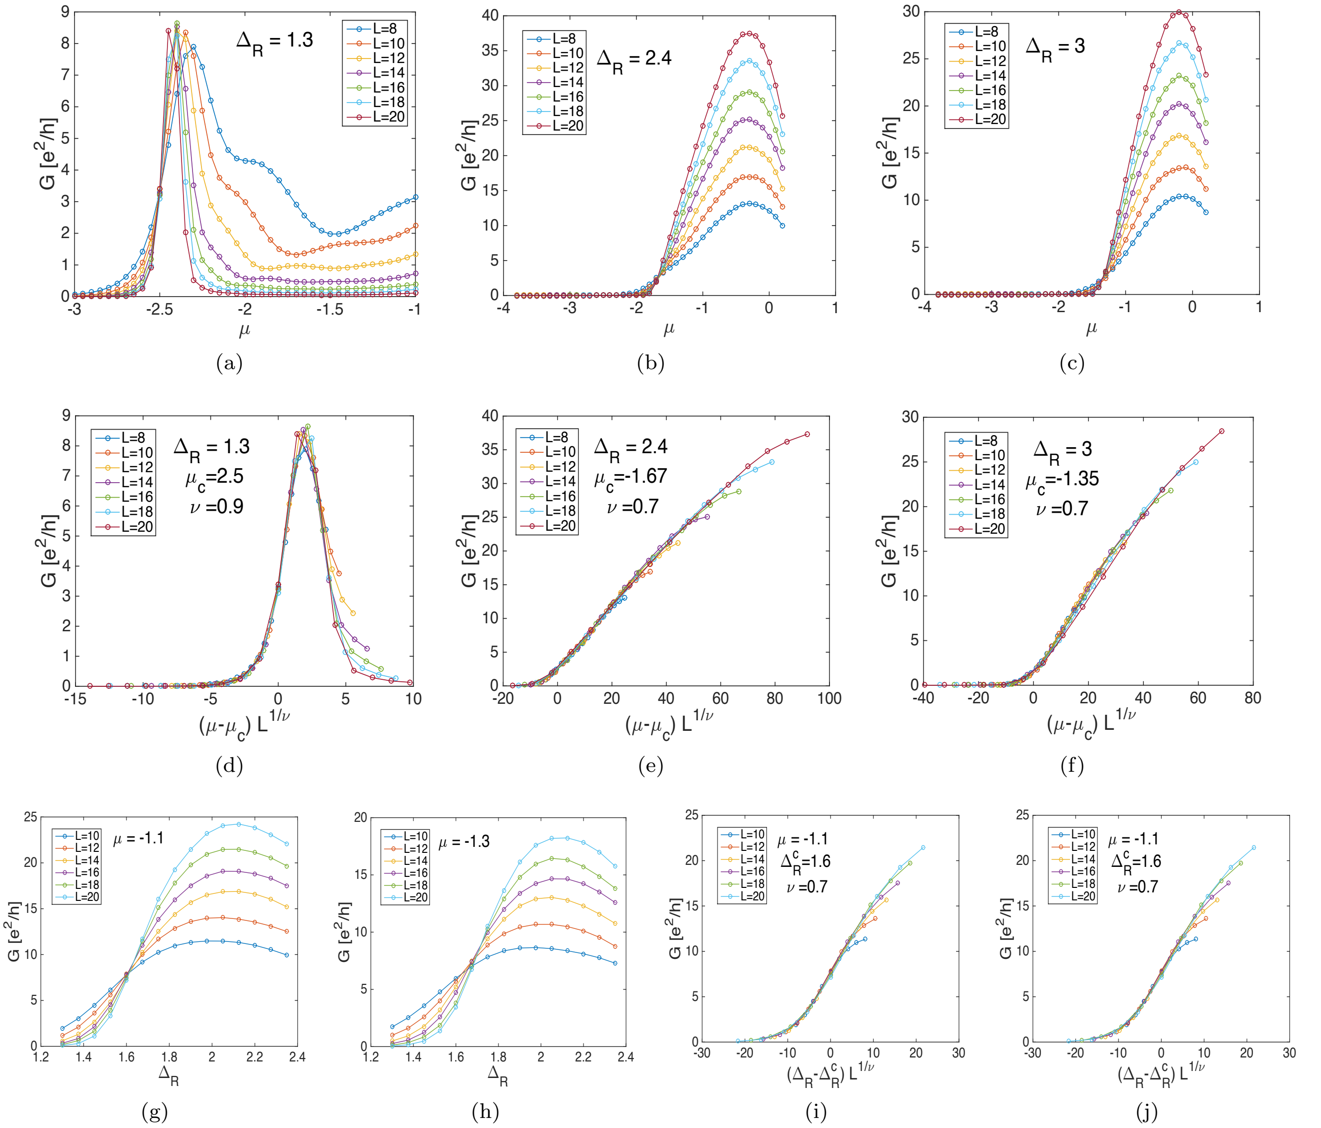


Figure 3: Normalized thermal conductance (NTC) $G$ (in units of $e^2/h$) across thermal insulator-insulator transition (IIT), tuned by random, but only the real component of the $s$-wave pairing (appearing as random chiral chemical potential) is shown in subfigures (a), (b) and (c). Corresponding data collapses are presented in (d), (e) and (f). NTC across metal-insulator transition (MIT) is shown in subfigures (g) and (h), and associated data collapses across MIT are displayed in (i) and (j). Location of the transition points, best fitting values of $\nu$ across IIT and MIT, system sizes are quoted inside the figures.

for a fixed value of $\Delta$ and for all different types of elastic scatter.

Before proceeding to additional numerical results we present some details of the numerical analysis. Note that electrical conductance $G$, measured in units of $e^2/h$ and thermal conductance $G_T$, measured in units of $G_0 = \frac{1}{2} \times \frac{\pi^2 k_B^2 T_0}{3h}$ are related to each other according to the Wiedemann-Franz law

$$\frac{G}{e^2/h} = \frac{G_T}{\pi^2 k_B^2 T_0/(6h)} \Rightarrow G_T = \frac{\pi^2 k_B^2 T_0}{6h} \times \frac{h}{e^2}\, G \Rightarrow G_T = \frac{\pi^2 k_B^2 T_0}{6e^2}\, G \Rightarrow G_T = \mathcal{L} G, \tag{12}$$

where $\mathcal{L} = \frac{\pi^2 k_B^2 T_0}{6e^2}$ is the Lorentz number, and $T_0$ is the temperature of the metallic reservoir, such that $T_0 \ll T_c$ (transition temperature for superconductivity). This connection between the electrical and thermal conductance allows us to compute a fictitious electrical conductance $G$ for topological superconductor, obtained by assuming particles and holes both carry the same electrical charge $e$. The electrical conductance is then related to the thermal

conductance according to $G_T = \mathcal{L}G$, as $T_0 \to 0$.

In this Supplementary Materials we also display the behavior of normalized thermal conductance($G$) across the transition between two topologically distinct thermal insulators, as well as themal metal-insulator transition, driven by random charge impurities (see Fig. 2) and the real component of $s$-wave pairing (see Fig. 3).

## V. CLASS DIII NEMATIC TOPOLOGICAL SUPERCONDUCTOR IN CU$_x$BI$_2$SE$_3$

The minimal model for $Bi_2Se_3$ is described by a four-component massive Dirac Hamiltonian

$$H_{\text{Bi}_2\text{Se}_3} = \sum_{\mathbf{k}} \Psi^\dagger_{\mathbf{k}} \hat{H}_{\text{Bi}_2\text{Se}_3}(\mathbf{k}) \Psi_{\mathbf{k}}, \tag{13}$$

where $\Psi_{\mathbf{k}}$ is a four-component spinor, defined as $\Psi^\top_{\mathbf{k}} = \left[c^\dagger_{1,\uparrow,\mathbf{k}}, c^\dagger_{1,\downarrow,\mathbf{k}}, c^\dagger_{2,\uparrow,\mathbf{k}}, c^\dagger_{2,\downarrow,\mathbf{k}}\right]$, and $c^\dagger_{j,s,\mathbf{k}}$ represents fermion creation operator in $j^{th}$ orbital, with spin projection $s = \uparrow / \downarrow$ and momentum $\mathbf{k}$. Here for simplicity we neglect the particle-hole anisotropy. The Hamiltonian operator reads as[7]

$$\hat{H}_{\text{Bi}_2\text{Se}_3}(\mathbf{k}) = v_\perp \left(k_x \Gamma_1 + k_y \Gamma_2\right) + v_z k_z \Gamma_3 + \Gamma_0 m - \mu I_4, \tag{14}$$

where the four component mutually anticommuting $\Gamma$ matrices are $\Gamma_1 = \eta_3 \otimes \sigma_2$, $\Gamma_2 = -\eta_3 \otimes \sigma_1$, $\Gamma_3 = \eta_2 \otimes \sigma_0$ and $\Gamma_0 = \eta_1 \otimes \sigma_0$ and $\Gamma_4 = \eta_3 \otimes \sigma_3$, and $I_4$ is the four dimensional identity matrix. The chemical potential is denoted by $\mu$, which lies in the conduction band $\mu > 0$. Two sets of Pauli matrices $\boldsymbol{\eta}$ and $\boldsymbol{\sigma}$ respectively operates on orbital and spin indices. The underlying crystallographic symmetry implies that $v_\perp \neq v_z$. To capture all possible local pairing in this model we need to perform Nambu doubling on the above Hamiltonian. Let us define a Nambu-doubled eight component spinor as $\Psi = \left[\Psi^\top_{p,\mathbf{k}}, \Psi^\top_{h,-\mathbf{k}}\right]$, where $\Psi^\top_{p,\mathbf{k}} = \Psi^\top_{\mathbf{k}}$ and $\Psi^\top_{h,-\mathbf{k}} = \Psi_{p,\mathbf{k}}$. In this basis the massive Nambu-Dirac Hamiltonian, corresponding to the one shown in Eq. (14), takes the form

$$\hat{H}^{ND}_{\text{Bi}_2\text{Se}_3}(\mathbf{k}) = v_\perp \left(k_x \tau_3 \otimes \Gamma_1 + k_y \tau_0 \otimes \Gamma_2\right) + v_z k_z \tau_3 \otimes \Gamma_3 + m \tau_3 \otimes \Gamma_0 - \mu \tau_3 \otimes I_4, \tag{15}$$

where the new set of Pauli matrices $\boldsymbol{\tau}$ operates on the Nambu index. All together one can write down six local pairing terms for such model and corresponding effective single particle Hamiltonian reads as

$$\hat{H}_{SC} = \left(\tau_1 \cos\phi + \tau_2 \sin\phi\right) \otimes \left[\Delta_s \Gamma_{42} + \Delta_p \Gamma_{02} + \Delta_1 \Gamma_3 + \Delta_2 \Gamma_{04} + \Delta_3 \Gamma_1 + \Delta_0 \Gamma_{13}\right], \tag{16}$$

where $\phi$ is the superconducting phase and $\Gamma_{jk} = i\Gamma_j\Gamma_k$. The amplitude of $s$-wave (singlet) and $p$-wave (triplet) pairing are respectibely given by $\Delta_s$ and $\Delta_p$, which respectively transform as scalar and pseudo-scalar under Lorentz transformation[8]. Remaining four pairings together constitute a *four-vector* under the Lorentz transformation and amplitude of its $\mu^{th}$ component is $\Delta_\mu$, where $\mu = 0, 1, 2, 3$. Transformation of above $6 \times 2 = 12$ pairing matrices under the time-reversal operation is shown in Table II. The time-reversal operator ($\mathcal{T}$) in the Nambu-Dirac basis reads as $\mathcal{T} = i\tau_0 \otimes (\eta_0 \otimes \sigma_2) \otimes K$, where $K$ is the complex conjugation and $\mathcal{T}^2 = -1$.

The $s$-wave pairing always gives rise to fully gapped spectrum, whereas with an underlying $p$-wave pairing there is a topological phase transition (through gap closing) at $\mu^2 + |\Delta_p|^2 = m^2$. Although on either side of this transition the spectrum is fully gapped, the paired state can be associated with a nontrivial integer $Z$ invariant only when $\mu^2 + |\Delta_p|^2 > m^2$. The time-like component of the vector pairing ($\mu = 0$) gives rise to a surface, supporting gapless excitation of BdG fermions in the momentum space. Thus such pairing is possibly not energetically favored over the rest and thus we do not discuss this pairing in any further details here. The space-like components of vector pairing $\Delta_j$ with $j = 1, 2, 3$ gives rise to nodal spectrum when $\mu^2 + |\Delta_j|^2 > m^2$, with the nodes being at $k_j = \pm\sqrt{|\Delta_j|^2 + \mu^2 - m^2}$. However, it is still conceivable to realize a fully, but anisotropic gapped spectrum from an appropriate linear combination of vector (space-like) pairings. In particular, two mutually anticommuting components of the $j^{th}$ and $k^{th}$ vector pairing, where $j \neq k$, can give rise to a fully gapped paired state, since individually they support two nodes along the $j$ and $k$ axis in the momentum space, respectively, while producing fully gapped spectrum in the rest of the Brillouin zone. For example, the time-reversal invariant components of $1^{st}$ and $2^{nd}$ vector pairing, respectively represented by the eight dimensional matrices $\tau_2 \otimes \Gamma_3$ and $\tau_1 \otimes \Gamma_{04}$ supports a fully gapped (anisotropic) spectrum

$$E_\alpha(\mathbf{k}) = \pm \left[\mathbf{k}^2 + m^2 + \mu^2 + |\Delta_1|^2 + |\Delta_2|^2 - 2\alpha\sqrt{\left(k_x|\Delta_1| + k_y|\Delta_2|\right)^2 + \mathbf{k}^2 + m^2\left(\mu^2 + |\Delta_1|^2 + |\Delta_2|^2\right)}\right]^{1/2} \tag{17}$$

| Pairing | Representation of $Bi_2$ $Se_3$ | Dirac basis after unitary rotation | Under $\mathcal{T}$ |
|---|---|---|---|
| S-wave (scalar) | $\tau_1 \otimes i\Gamma_4\Gamma_2$ | $\tau_1 \otimes \alpha_1\alpha_3$ | X |
| | $\tau_2 \otimes i\Gamma_4\Gamma_2$ | $\tau_1 \otimes \alpha_1\alpha_3$ | ✓ |
| odd parity (pseudo scalar) | $\tau_1 \otimes i\Gamma_0\Gamma_2$ | $\tau_2 \otimes \alpha_2$ | ✓ |
| | $\tau_2 \otimes i\Gamma_0\Gamma_2$ | $\tau_1 \otimes \alpha_2$ | X |
| $1^{st}$ component of vector pairing | $\tau_1 \otimes \Gamma_3$ | $\tau_2 \otimes i\alpha_3\beta$ | X |
| | $\tau_2 \otimes \Gamma_3$ | $\tau_1 \otimes i\alpha_3\beta$ | ✓ |
| $2^{nd}$ component of vector pairing | $\tau_1 \otimes i\Gamma_0\Gamma_4$ | $\tau_2 \otimes \Gamma_5$ | ✓ |
| | $\tau_2 \otimes i\Gamma_0\Gamma_4$ | $\tau_1 \otimes \Gamma_5$ | X |
| $3^{rd}$ component of vector pairing | $\tau_1 \otimes \Gamma_1$ | $\tau_2 \otimes i\alpha_1\beta$ | X |
| | $\tau_2 \otimes \Gamma_1$ | $\tau_1 \otimes i\alpha_1\beta$ | ✓ |
| $0^{th}$ component of vector pairing | $\tau_1 \otimes i\Gamma_1\Gamma_3$ | $\tau_1 \otimes i\alpha_2\beta$ | X |
| | $\tau_2 \otimes i\Gamma_1\Gamma_3$ | $\tau_2 \otimes i\alpha_2\beta$ | ✓ |

Table II: Various possible pairings in a time-reversal and inversion symmetric narrow gap semiconductors, such as $Cu_xBi_2Se_3$, their transformation under the unitary rotation by $U$ and the reversal of time ($\mathcal{T}$). Here the symbols ✓ and $\times$ respectively correspond to even and odd.

when $\mu^2 + |\Delta_1|^2 + |\Delta_2|^2 > m^2$. Here each band is Kramers degenerate, $\alpha = \pm$ and we have dropped $v_\perp, v_z$ for notational simplicity. Since these superconductors break rotational symmetry, we name them *nematic superconductors*. Next, we will show that when such combination of two pairings is projected onto the Fermi surface, the reduced BCS Hamiltonian assumes the form of a topological pairing in class DIII.

To carry out this exercise, we first perform a unitary transformation $U^\dagger \, \hat{H}^{ND}_{\mathrm{Bi_2Se_3}}(\mathbf{k})\, U$, where $U$ is an eight dimensional unitary matrix $U = U_p \oplus (U_p\beta)$, with

$$U_p = \frac{1}{\sqrt{2}} \begin{pmatrix} i & 0 & 1 & 0 \\ 0 & i & 0 & -1 \\ i & 0 & -1 & 0 \\ 0 & i & 0 & 1 \end{pmatrix}, \ \beta = \begin{pmatrix} \sigma_0 & 0 \\ 0 & -\sigma_0 \end{pmatrix}, \text{ and } \Gamma_5 = \begin{pmatrix} 0 & -i\sigma_0 \\ i\sigma_0 & 0 \end{pmatrix}, \ \alpha_j = \begin{pmatrix} 0 & \sigma_j \\ \sigma_j & 0 \end{pmatrix}, \tag{18}$$

for $j = 1, 2, 3$, after which

$$U^\dagger \, \hat{H}^{ND}_{\mathrm{Bi_2Se_3}}(\mathbf{k})\, U = (\tau_0 \otimes \alpha_1)\ k_x + (\tau_3 \otimes \alpha_2)\ k_y + (\tau_0 \otimes \alpha_3)\ k_z + (\tau_3 \otimes \beta)\ m - (\tau_3 \otimes I_4)\ \mu \equiv H_{ND}(\mathbf{k}). \tag{19}$$

$H_{ND}(\mathbf{k})$ is the standard nambu-Dirac Hamiltonian. For notational simplicity we have dropped the Fermi velocities $v_\perp$ and $v_z$ in Eq. (19). Transformations of various pairing matrices, shown in Eq. (16), under the unitary transformation, which leaves the time-reversal operator *unchanged*, are shown in Table II. *Our formalism can be adopted to address pairing properties in narrow gap semiconductors. The only task is to find the appropriate unitary transformation (U) that will produce the standard Nambu-Dirac Hamiltonian, displayed in Eq. (19).* Diagonalizing the above Hamiltonian with the diagonalizer[9]

$$\mathcal{D} = \begin{bmatrix} \frac{k_x - ik_y}{\sqrt{2\lambda(\lambda-m)}} & \frac{k_z}{\sqrt{2\lambda(\lambda-m)}} & \frac{-k_x+ik_y}{\sqrt{2\lambda(\lambda+m)}} & \frac{-k_z}{\sqrt{2\lambda(\lambda+m)}} \\ \frac{-k_z}{\sqrt{2\lambda(\lambda-m)}} & \frac{k_x+ik_y}{\sqrt{2\lambda(\lambda-m)}} & \frac{k_z}{\sqrt{2\lambda(\lambda+m)}} & \frac{-k_x-ik_y}{\sqrt{2\lambda(\lambda+m)}} \\ 0 & \frac{\lambda-m}{\sqrt{2\lambda(\lambda-m)}} & 0 & \frac{\lambda+m}{\sqrt{2\lambda(\lambda+m)}} \\ \frac{\lambda-m}{\sqrt{2\lambda(\lambda-m)}} & 0 & \frac{\lambda+m}{\sqrt{2\lambda(\lambda+m)}} & 0 \end{bmatrix}, \tag{20}$$

where $\lambda = \sqrt{\mathbf{k}^2 + m^2}$, we find

$$\mathcal{D}^\dagger H_{ND}(\mathbf{k}) \mathcal{D} = \begin{pmatrix} \left(\sqrt{\mathbf{k}^2+m^2} - \mu\right)\ \sigma_0 & 0 & 0 & 0 \\ 0 & \left(-\sqrt{\mathbf{k}^2+m^2} - \mu\right)\ \sigma_0 & 0 & 0 \\ 0 & 0 & -\left(\sqrt{\mathbf{k}^2+m^2} - \mu\right)\ \sigma_0 & 0 \\ 0 & 0 & 0 & \left(\sqrt{\mathbf{k}^2+m^2} + \mu\right)\ \sigma_0 \end{pmatrix}. \tag{21}$$

The first and third entries correspond to the energy of the Kramers degenerate conduction band, while the second and forth entries correspond to the energy of the valence band (also Kramers degenerate). Now, completely neglecting the contribution from the filled valence band (assuming $\mu > 0$), we obtain the kinetic energy in the vicinity of the Fermi surface (located within the conduction band) to be

$$H_0 = \begin{pmatrix} \left(\sqrt{\mathbf{k}^2 + m^2} - \mu\right)\, \sigma_0 & 0 \\ 0 & -\left(\sqrt{\mathbf{k}^2 + m^2} - \mu\right)\, \sigma_0 \end{pmatrix} \approx \begin{pmatrix} \left[\frac{\mathbf{k}^2}{2m} - \mu\right]\, \sigma_0 & 0 \\ 0 & -\left[\frac{\mathbf{k}^2}{2m} - \mu\right]\, \sigma_0 \end{pmatrix}, \tag{22}$$

in the four component spinor basis $\Psi^\dagger_{\mathbf{k}} = \left(c^*_{\uparrow,\mathbf{k}}, c^*_{\downarrow,\mathbf{k}}, c_{\downarrow,-\mathbf{k}}, -c_{\uparrow,-\mathbf{k}}\right)$, where $c^*_{s,\mathbf{k}}$, $c_{s,\mathbf{k}}$ are respectively quasiparticle creation and annihilation operators with momentum $\mathbf{k}$, and spin projection $s =\uparrow / \downarrow$ near the Fermi surface. Applying the diagonalizing matrix on the real component of various triplet pairings (except the $0^{th}$ component of $\Delta_\mu$) we obtain

$$\begin{aligned} \Delta_p\ (\tau_2 \otimes \alpha_2) &\to \frac{\Delta_p}{k_F} \left[\begin{array}{c|c} 0 & -\sigma_1 k_x + \sigma_2 k_y + \sigma_3 k_z \\ \hline H.c. & 0 \end{array}\right], \quad \Delta_1\ (\tau_1 \otimes i\alpha_3\beta) \to \frac{\Delta_1}{k_F} \left[\begin{array}{c|c} 0 & -\sigma_2 k_z + \sigma_3 k_y \\ \hline H.c. & 0 \end{array}\right], \\ \Delta_2\ (\tau_2 \otimes \Gamma_5) &\to \frac{\Delta_2}{k_F} \left[\begin{array}{c|c} 0 & -\sigma_1 k_z - \sigma_3 k_x \\ \hline H.c. & 0 \end{array}\right], \quad \Delta_3\ (\tau_1 \otimes i\alpha_1\beta) \to \frac{\Delta_3}{k_F} \left[\begin{array}{c|c} 0 & -\sigma_1 k_y - \sigma_2 k_x \\ \hline H.c. & 0 \end{array}\right], \end{aligned} \tag{23}$$

after completely neglecting the contribution from the filled valence band, where $k_F$ is Fermi momentum. The form of triplet $p$-wave pairing has already been announced in the main part of the paper. Interestingly, when the real components of two vector pairings ($1^{st}$ and $2^{nd}$ component of $\Delta_\mu$) coexist the resulting reduced BCS Hamiltonian

$$H_v = \left(\frac{\mathbf{k}^2}{2m} - \mu\right) \left(\begin{array}{c|c} \sigma_0 & 0 \\ \hline 0 & -\sigma_0 \end{array}\right) + \Delta_2\, \frac{k_z}{k_F} \left(\begin{array}{c|c} 0 & \sigma_1 \\ \hline \sigma_1 & 0 \end{array}\right) - \Delta_1\, \frac{k_z}{k_F} \left(\begin{array}{c|c} 0 & \sigma_2 \\ \hline \sigma_2 & 0 \end{array}\right) + \left(\Delta_2\, \frac{k_x}{k_F} + \Delta_1\, \frac{k_y}{k_F}\right) \left(\begin{array}{c|c} 0 & \sigma_3 \\ \hline \sigma_3 & 0 \end{array}\right), \tag{24}$$

also assumes the form of a topological superconductor in class DIII[10].

---

[1] P. Goswami, and S. Chakravarty, Phys. Rev. Lett. **107**, 196803 (2011).
[2] J. A. Gracey, Nucl. Phys. B **367**, 657 (1991).
[3] C. Luperini, and P. Rossi, Annals of Physics **212**, 371 (1991).
[4] N. A. Kivel, A. A. Stepanenko, and A. N. Vasil'ev, Nucl. Phys. B **424**, 619 (1994).
[5] M. Moshe, and J. Zinn-Justin, Physics Reports **385**, 69 (2003).
[6] B. Roy, and S. Das Sarma, Phys. Rev. B **90**, 241112(R) (2014).
[7] L. Fu, and E. Berg, Phys. Rev. Lett. **105**, 097001 (2010).
[8] T. Ohsaku, Phys. Rev. B **65**, 024512 (2002).
[9] A. P. Schnyder, S. Ryu, A. Furusaki, A. W. W. Ludwig, Phys. Rev. B **78**, 195125 (2008).
[10] See also J. W. F. Venderbos, V. Kozii, L. Fu, Phys. Rev. B **94**, 180504(R) (2016).
